# Supplementary material for: SAFE^d: Self-Attestation For Networks of Heterogeneous Embedded Devices
Source: arXiv:1909.08168 source file (2019-12-12)
Supplement: Supplementary file 1 [file appendix.tex]

%\newpage
\appendix
\section{Attestation Algorithm}
\label{apx:attestation-algorithm}

\begin{algorithm}[t]
	\begin{algorithmic}[1]
		\Variables
		\State attest\_in\_progress: \emph{true} if an attestation is in progress
		\State UID: the ID of the \emph{proof} under attestation
		\State hash: the value measured by the \emph{Prover}
		\State proof[O] = \{\emph{Null}\}, the \emph{proof} extracted by the \emph{overlay} O
		\EndVariables
		\Function{engage\_attestation}{}
		
		\If{attest\_in\_progress}\label{lst:algorithm:1}
		
		\State \Call{validate\_hash}{}
		\Else
		\State attest\_in\_progress $\gets$ \emph{true} \label{lst:algorithm:4}
		\State $\text{OID}_\text{R} \gets$ \Call{generate\_random\_oid}{} \label{lst:algorithm:2}
		\State prv $\gets$ \Call{get\_successor}{$\text{OID}_\text{R}$} \label{lst:algorithm:3}
%		\State UID $\gets$ \Call{get\_uid}{prover} \label{lst:algorithm:5}
		\State (UID, hash) $\gets$ \Call{engage\_prover}{prv} \label{lst:algorithm:6}
		\State \Call{validate\_hash}{}
		\EndIf
		\EndFunction
		
		\Function{validate\_hash}{}
		
		\State $p \gets$ \Call{get\_proof}{UID} \label{lst:algorithm:7}
		\If{p = \emph{Null}}
		
		\State proof[O] $\gets$ \emph{no-proof} \label{lst:algorithm:8}
		\ElsIf{timeout}
		
		\State proof[O] $\gets$ \emph{timeout} \label{lst:algorithm:9}
		\Else
		
		\State proof[O] $\gets$ \emph{p} \label{lst:algorithm:10}
		\EndIf
		
		\If{$\forall p \in \text{proof},~p != \emph{Null}$} \label{lst:algorithm:11}
		\State \Call{voting\_and\_recovery}{} \label{lst:algorithm:12}
		\State attest\_in\_progress $\gets$ \emph{false}
		\EndIf
		\EndFunction
		\caption{Attestation Pseudo-code}
		\label{alg:attesation}
	\end{algorithmic}
\end{algorithm}

Algorithm~\ref{alg:attesation} shows the $\text{SAFE}^d$ attestation pseudo-code.
$\text{SAFE}^d$ extends the classic attestation paradigm (Section~\ref{ssec:remote-attestation}) 
by allowing all devices being both \emph{Prover} and \emph{Verifier}.
The actual role is randomly assigned at run-time.
In our proof-of-concept, we implemented the attestation phase as an extra 
operation that is randomly triggered with 
\emph{stabilize} and \emph{rectify}. The device starts performing attestations
when it reaches \emph{member-and-running} status.
Since the entire $\text{SAFE}^d$ algorithm is implemented in the trusted anchor (Section~\ref{sec:implementation}),
 and the
messages are encrypted (Section~\ref{ssec:secure-device-comm}), an attacker
cannot precisely block the attestation phase without affecting the
entire network.

The attestation is a collaborative operation which is performed by each
\emph{overlay} independently. Therefore, we use global variables for avoiding concurrency issues.
The process is implemented by two routines:
\begin{enumerate*}[label=(\roman*)]
	\item \texttt{ENGAGE\_ATTESTATION} that sends a challenge to the \emph{Prover}, and
	\item \texttt{VALIDATE\_HASH} that validates the hash received.
\end{enumerate*}
Each overlay can autonomously start an attestation by triggering
\texttt{ENGAGE\_ATTESTATION}, whose duty is to identify a random device to attest.
The function verifies if another \emph{overlay} has already started an attestation
by testing the flag \texttt{attest\_in\_progress} (Line~\ref{lst:algorithm:1}).
If the variable is set to \emph{true}, the device invokes \texttt{VALIDATE\_HASH}.
Otherwise, it starts a new attestation. In this case, it sets
\texttt{attest\_in\_prog\\ress} to \emph{true}, 
thus blocking other \emph{overlays} starting a
new attestation (Line~\ref{lst:algorithm:4}).
Then, it randomly selects a \emph{Prover} (Line~\ref{lst:algorithm:2}-\ref{lst:algorithm:3}),
and engages the \emph{Prover} itself (Line~\ref{lst:algorithm:6}).
\texttt{ENGANGE\_PROVER} sends a \emph{nonce} and waits for the HASH.
Finally, UID and \emph{hash} are stored in global variables while waiting for other
\emph{overlays} to verify their correctness.

After retrieving an \emph{hash}, \texttt{VALIDATE\_HASH} function 
retrieves the \emph{proofs} from the other \emph{overlays},
and stores them in the global variable \emph{proof} (Label~\ref{lst:algorithm:7}). 
Here, we handle three cases:
\begin{itemize}
	\item it does not receive any \emph{proof} (Line~\ref{lst:algorithm:8}).
	\item it gets a timeout (Line~\ref{lst:algorithm:9}).
	\item it obtains a \emph{proof} (Line~\ref{lst:algorithm:10}).
\end{itemize}
When all \emph{overlays} fetch a \emph{proof} (Line~\ref{lst:algorithm:11}), 
then we use a voting system to check its correctness (Line~\ref{lst:algorithm:12}).
The algorithm follows three main steps:
\begin{enumerate*}[label=(\roman*)]
	\item decide the correct \emph{proof} by majority,
	\item we perform a recovery on those \emph{overlays} with \emph{timeouts} or
	\emph{no-proof},
	\item the devices which returned incoherent \emph{proofs} are considered corrupted.
\end{enumerate*}
In case the \emph{proofs} are not enough to elect the correct one,
we consider the entire network as corrupted.
The voting system follows the same rule of Bizantine-fault-tolerance~\cite{Castro:2002:PBF:571637.571640},
therefore, $\text{SAFE}^d$ can support up to one third of corrupted devices.
